# Supplementary material for: Dynamical local connector approximation for electron addition and removal spectra
Source: arXiv:1708.02450 ancillary file (2017-08-09)
Supplement: Supplementary file 1 [file sup_mat.pdf]

# Supplemental Material for
# Dynamical local connector approximation for electron addition and removal spectra

Marco Vanzini,[1,2,*] Lucia Reining,[1,2] and Matteo Gatti[1,2,3]
[1]*Laboratoire des Solides Irradiés, École Polytechnique, CNRS, CEA, Université Paris-Saclay, F-91128 Palaiseau, France*
[2]*European Theoretical Spectroscopy Facility (ETSF)*
[3]*Synchrotron SOLEIL, L'Orme des Merisiers, Saint-Aubin, BP 48, F-91192 Gif-sur-Yvette, France*
(Dated: August 4, 2017)

In this Supplemental material we present some additional information for the interested reader. In Sec. I we describe how to obtain the spectral potential (SP) in the homogeneous electron gas (HEG) in practice, for any approximation to the self–energy; then, we will consider in detail the band structure obtained through the SP, and explain how two different band structures (BS) can lead to the same spectral function (SF). Finally, we will show how it is possible, through the addition of a function $\Delta(\omega)$, to obtain both the SF and the BS via a local SP. In Sec. II we give a more formal derivation of the shift of frequency arguments in the "connector" that we use in the text. In Sec. III we present the results of our dynamical local connector approximation (dynLCA) applied to aluminum: the behavior is qualitatively similar to sodium. In Sec. IV we discuss the necessity of going beyond simpler connectors. Finally, in Sec. V we report some technical details that are needed to perform the calculations we discuss in the paper.

## I. HEG AS A MODEL SYSTEM

We consider in more detail the SP in the HEG; here, any local quantity is constant in real space, and the local SF is a function of frequency only. If the exchange-correlation (xc) self-energy (SE) is real and static, the SF evaluated through it can be written as:

$$A(\omega) \equiv \sum_{\boldsymbol{k}} \delta\left(\omega - \varepsilon_{\boldsymbol{k}}\right) = \int_0^{+\infty} \frac{dk}{2\pi^2} k^2 \delta\left(\omega - \varepsilon_k\right),$$

where $\varepsilon_k = \varepsilon_k^0 + \Sigma^h(k)$. Calling $k^0(\omega)$ the only solution (if $\omega \geq \Sigma^h(k=0)$; otherwise, $A(\omega) = 0$) to the quasiparticle (QP) equation $\omega = \varepsilon_k^0 + \Sigma^h(k)$, the delta function can be simplified and the SF becomes:

$$A(\omega) = \int_0^{+\infty} \frac{dk}{2\pi^2} \frac{k^2}{\left|k + d\Sigma^h(k)/dk\right|} \delta\left(k - k^0(\omega)\right) = \\ = \frac{1}{2\pi^2} \left. \frac{k^2}{\left|k + \Sigma^{h'}(k)\right|} \right|_{k=k^0(\omega)},$$

where in the last line $\Sigma^{h'}$ is the shorthand notation for the derivative $d\Sigma^h/dk$. On the other hand, since the SP depends only on frequency, the SF in the auxiliary system is given by:

$$A_{\mathrm{SF}}(\omega) = \int_0^{+\infty} \frac{dk}{2\pi^2} k^2 \delta\left(\omega - \varepsilon_k^0 - v_{\mathrm{SF}}^h(\omega)\right) = \\ = \frac{1}{2\pi^2} \sqrt{2\left[\omega - v_{\mathrm{SF}}^h(\omega)\right]} \qquad (1)$$

with $\omega \geq v_{\mathrm{SF}}^h(\omega)$, and zero otherwise. By equating the two, one obtains the exact expression of the SP for a real and static self-energy in the HEG:

$$v_{\mathrm{SF}}^h(\omega) = \omega - 2\left[\frac{\frac{k^2}{2}}{k + \Sigma^{h'}(k)}\right]^2_{k=k^0(\omega)}, \qquad (2)$$

which is valid for $\omega \geq \Sigma^h(k=0)$. When the SF is zero, the SP is undetermined, and we define it to be the constant $\Sigma^h(k=0)$, so that the whole SP is a continuous function of $\omega$. Its dependence on the density of the HEG enters through the Fermi energy in $\Sigma^h$ and in $k^0(\omega)$.

Note that this procedure is in principle equivalent to a self-consistent solution of the generalized Sham-Schlüter equation[1,2]. With this potential at hand, the SF is exactly reproduced, as can be seen from Fig. I, central panel.

**The band structure.** On the other hand, the BS (right panel of the same figure) – or equivalently the dispersion relation (left panel) – differs from the one evaluated through the SE by the positive quantity $\Delta^h(\omega)$ defined in the main article (which is zero only at $\Gamma$ and for $|\boldsymbol{k}| \to \infty$): even in the model system, where we obtain by definition (and analytically) the exact SF, the BS differs from the exact one.

The fact that two different BSs can lead to the same SF can be understood from the formula relating the BS to the SF: in the usual SE approach, the expression for the SF can be rewritten as:

$$A(\omega) = \int_0^{+\infty} \frac{dk}{2\pi^2} \frac{k^2}{\left|k + \Sigma^{h'}(k)\right|} \delta\left(k - k^0(\omega)\right).$$

The same is true in the SP approach, where the role of $\Sigma^h(k)$ is played by $v_{\mathrm{SF}}^h(\omega)$; since the latter is $k$-independent, the amplitude of each delta peak will be $k$ instead of $k^2/|k+\Sigma^{h'}(k)|$, and $k^0(\omega)$ will be replaced by the positive solution of the QP equation $\omega = \varepsilon_k^0 + v_{\mathrm{SF}}^h(\omega)$, namely $k_{\mathrm{SF}}^0(\omega) = \sqrt{2\left[\omega - v_{\mathrm{SF}}^h(\omega)\right]}$:

$$A_{\mathrm{SF}}(\omega) = \int_0^{+\infty} \frac{dk}{2\pi^2} k\, \delta\left(k - k_{\mathrm{SF}}^0(\omega)\right).$$

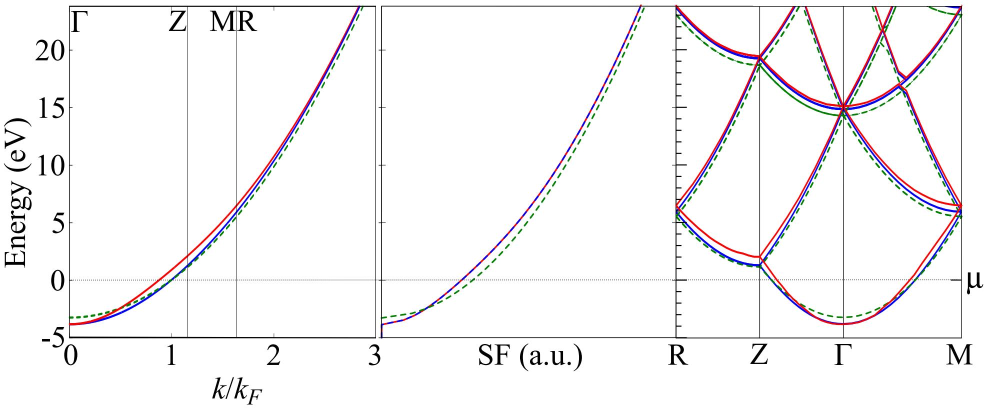


FIG. 1: HEG ($r_s = 3.9315 a_0$, Na average value) dispersion (left), spectral function (middle) and band structure (right), analytic results. The blue curve has been calculated using the SE, while the red one is our SP approach (as a comparison, the green-dashed curve for LDA-KS). The high symmetry points in the BS refer to a simple cubic unit cell: R $= \left(0, \frac{1}{2}, \frac{1}{2}\right)$, Z $= \left(0, 0, \frac{1}{2}\right)$, $\Gamma = (0, 0, 0)$ and M $= \left(\frac{1}{2}, \frac{1}{2}, 0\right)$.

In a discrete system, in order for the two SFs $A(\omega)$ and $A_{\mathrm{SF}}(\omega)$ to be the same, it is enough that the amplitude *and* the position of each delta peak be the same: from the position requirement $k^0_{\mathrm{SF}}(\omega) = k^0(\omega)$ we automatically would obtain the expected BS.

For a continuous spectrum, instead, the sum over $k$ spans the same whole positive axis, and only the amplitude of each delta peak becomes relevant: this is, on the one hand (SE approach), a non-trivial amplitude given by $k^2/|k + \Sigma^{h'}(k)|$, while on the other hand (SP approach), a free-electron like amplitude given by $k$, where the two $k$s are set by the respective delta functions to $k^0(\omega)$ and $k^0_{\mathrm{SF}}(\omega)$. If one requires the two amplitudes to be the same for each value of $\omega$, one immediately faces the fact that the two $k$s cannot have the same value, since they are related by:

$$\left.\frac{k^2}{|k + \Sigma^{h'}(k)|}\right|_{k=k^0(\omega)} = k^0_{\mathrm{SF}}(\omega), \tag{3}$$

which allows the solution $k^0_{\mathrm{SF}}(\omega) = k^0(\omega)$ only in the particular cases $k = 0$ and $k \to \infty$.

In other words, one cannot reproduce the SF of an interacting HEG with a purely frequency dependent potential, and at the same time also reproduce the BS – at least if one keeps the prescription (1) for the calculation of the SF, as we will discuss now.

**The $\Delta$-correction.** Indeed, by changing the way $A(\omega)$ is calculated, it is possible to reproduce the SF *and* the BS with a local, frequency dependent potential. The reasoning is as follows:

The equivalent of Eq. (3) at fixed $k$ is the set of QP equations:

$$\begin{aligned} \varepsilon_k &= \varepsilon^0_k + \Sigma^h(k) \\ \varepsilon^{SF}_k &= \varepsilon^0_k + v^h_{\mathrm{SF}}\left(\varepsilon^{\mathrm{SF}}_k\right) \end{aligned}$$

where the first relation sets the reference BS (blue curves in Fig. I, left and right panels), and the second one is our approach (red curves). The difference between the two is $\Delta^h_k := \varepsilon^{\mathrm{SF}}_k - \varepsilon_k$, which can be re-expressed as a function of $\omega$ due to the one-to-one correspondence between $\omega$ and $k$ proper of the HEG: $\Delta^h(\omega) = v^h_{\mathrm{SF}}(\omega) - \Sigma^h\left(k^0(\omega)\right)$. These quantities are shown in Fig. 2.

By construction, shifting the SP to $v^h_{\mathrm{SF}}(\omega) - \Delta^h(\omega)$ will directly lead to the expected BS, since:

$$v^h_{\mathrm{SF}}\left(\varepsilon^{\mathrm{SF}}_k\right) - \Delta^h\left(\varepsilon^{\mathrm{SF}}_k\right) = \Sigma^h\left(k^0\left(\varepsilon^{\mathrm{SF}}_k\right)\right) \equiv \Sigma^h(k).$$

However, only the original $v^h_{\mathrm{SF}}(\omega)$ is the solution to Eq. (2), so Eq. (1) cannot yield anymore the correct SF. On the other side, with the correct BS at hand we can calculate the SF directly from $A_{\mathrm{SF}}(\omega) = \sum_k \delta\left(\omega - \varepsilon^{\mathrm{SF}}_k\right)$. Note that this *not* equivalent to using $A_{\mathrm{SF}}(\omega) = \sum_k \delta\left(\omega - \varepsilon_k(\omega)\right)$. With the former choice, the SF becomes equal to the reference one, since $\varepsilon^{\mathrm{SF}}_k = \varepsilon_k$ by construction.

With such a procedure, we obtain a new SP $\left(v^h_{\mathrm{SF}}(\omega) - \Delta^h(\omega)\right)$, through which, in the model system, both BS and SF are exactly reproduced.

## II. DERIVATION OF THE FREQUENCY SHIFT IN THE CONNECTOR

In this section, we present a rigorous derivation of Eq. (2) of the main text.

The auxiliary system GFs for the solid and for the model are $G_{\mathrm{SF}}$ and $G^h_{\mathrm{SF}}$ respectively. They can be derived from the same non-interacting GF $G_0$ via the following inverted Dyson equations:

$$\begin{aligned} G^{-1}_{\mathrm{SF}}(\boldsymbol{r}, \boldsymbol{r}', \omega) &= G^{-1}_0(\boldsymbol{r}, \boldsymbol{r}', \omega) - \Big[v_{\mathrm{e}}(\boldsymbol{r}) + \\ &\quad + v_{\mathrm{H}}(\boldsymbol{r}) + v_{\mathrm{SF}}(\boldsymbol{r}, \omega)\Big]\delta(\boldsymbol{r} - \boldsymbol{r}') \\ G^{h^{-1}}_{\mathrm{SF}}(\boldsymbol{r}, \boldsymbol{r}', \omega) &= G^{-1}_0(\boldsymbol{r}, \boldsymbol{r}', \omega) - v^h_{\mathrm{SF}}(\omega)\,\delta(\boldsymbol{r} - \boldsymbol{r}'). \end{aligned} \tag{4}$$

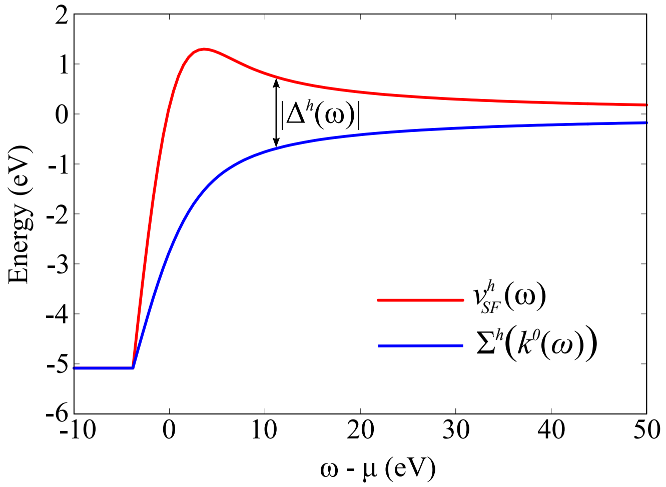


FIG. 2: HEG ($r_s = 3.9315a_0$) SP $v^h_{\mathrm{SF}}(\omega)$ and SE $\Sigma^h\left(k^0(\omega)\right)$ as a function of frequency (in eV, with $\mu = 0$). The difference between the two is the function $\Delta^h(\omega)$.

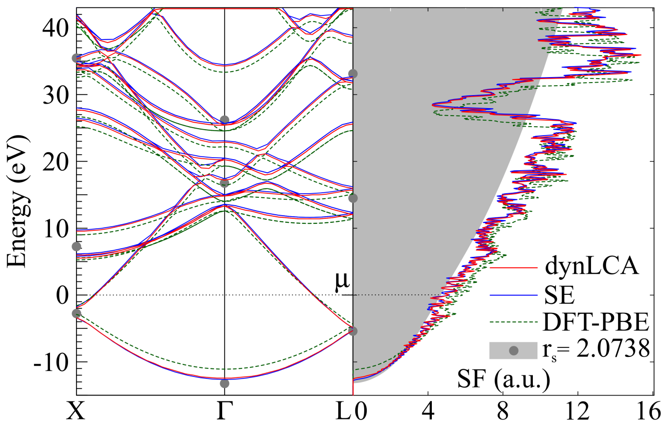


FIG. 3: Aluminum band structure (left) and SF (right). The blue curve is the SE calculation, while the red one is the dynLCA result, Eq. (4) with eq. (6) of the main article. As a comparison, the green-dashed curve for DFT-PBE; shaded area and gray dots for a SE calculation on a HEG of $r_s = 2.0738a_0$.

These relations are in principle exact. If we now require a connection between $v_{\mathrm{SF}}(\boldsymbol{r},\omega)$ and $v^h_{\mathrm{SF}}(\omega)$, that is if we ask the former to be derivable from the latter, there must be a real $c(\boldsymbol{r},\omega)$ that reshapes the HEG SF to account for lattice-related properties:

$$A^h_{\mathrm{SF}|n^h}(\boldsymbol{r},\omega - c(\boldsymbol{r},\omega)) = A(\boldsymbol{r},\omega). \qquad (5)$$

How does this requirement translate into the potentials? The answer can be found by implementing the relations (4) into eq. (5), assuming the following rule for shifting the frequency argument of $G_0^{-1}$:

$$G_0^{-1}(\boldsymbol{r},\boldsymbol{r}',\omega - c(\boldsymbol{r},\omega)) = G_0^{-1}(\boldsymbol{r},\boldsymbol{r}',\omega) - c(\boldsymbol{r},\omega)\,\delta(\boldsymbol{r}-\boldsymbol{r}'),$$

where $G_0^{-1}(\boldsymbol{r},\boldsymbol{r}',\omega) = \delta(\boldsymbol{r}-\boldsymbol{r}')\left[\omega - \left(-\frac{\nabla^2}{2}\right)\right]$. The previous equation is exact in the HEG, and we implement it in the real system by localizing $c$ in the spirit of the LDA. Using this relation, one can bypass $G_0^{-1}$ from eq. (4) and directly relate $G^{-1}_{\mathrm{SF}}(\boldsymbol{r},\boldsymbol{r}',\omega)$ to $G^{h^{-1}}_{\mathrm{SF}}(\boldsymbol{r},\boldsymbol{r}',\omega - c(\boldsymbol{r},\omega))$:

$$G^{-1}_{\mathrm{SF}}(\boldsymbol{r},\boldsymbol{r}',\omega) = G^{h^{-1}}_{\mathrm{SF}}(\boldsymbol{r},\boldsymbol{r}',\omega - c(\boldsymbol{r},\omega)) + \\ - \Big\{ v_{\mathrm{e}}(\boldsymbol{r}) + v_{\mathrm{H}}(\boldsymbol{r}) + v_{\mathrm{SF}}(\boldsymbol{r},\omega) + \\ - c(\boldsymbol{r},\omega) - v^h_{\mathrm{SF}}(\boldsymbol{r},\omega - c(\boldsymbol{r},\omega)) \Big\}\delta(\boldsymbol{r}-\boldsymbol{r}').$$

Inverting this equation, we obtain a Dyson-like equation between $G_{\mathrm{SF}}$ and $G^h_{\mathrm{SF}}$:

$$G_{\mathrm{SF}}(\boldsymbol{r},\boldsymbol{r}',\omega) = G^h_{\mathrm{SF}}(\boldsymbol{r},\boldsymbol{r}',\omega - c(\boldsymbol{r},\omega)) + \\ + \int d\boldsymbol{r}'' G^h_{\mathrm{SF}}(\boldsymbol{r},\boldsymbol{r}'',\omega - c(\boldsymbol{r},\omega)) \Big\{ v_{\mathrm{SF}}(\boldsymbol{r}'',\omega) + \\ - v^h_{\mathrm{SF}}(\omega - c(\boldsymbol{r}'',\omega)) - c(\boldsymbol{r}'',\omega) + v_{\mathrm{e}}(\boldsymbol{r}'') + \\ + v_{\mathrm{H}}(\boldsymbol{r}'') \Big\} G_{\mathrm{SF}}(\boldsymbol{r}'',\boldsymbol{r}',\omega).$$

From this expression and the definition of the SF, eq.(5) can be written as:

$$0 = \int d\boldsymbol{r}'' \Big\{ v_{\mathrm{SF}}(\boldsymbol{r}'',\omega) - v^h_{\mathrm{SF}}(\omega - c(\boldsymbol{r}'',\omega)) + \\ - c(\boldsymbol{r}'',\omega) + v_{\mathrm{e}}(\boldsymbol{r}'') + v_{\mathrm{H}}(\boldsymbol{r}'') \Big\} \times \\ \times \mathrm{Im}\left[ G^h_{\mathrm{SF}}(\boldsymbol{r},\boldsymbol{r}'',\omega - c(\boldsymbol{r},\omega))\, G_{\mathrm{SF}}(\boldsymbol{r}'',\boldsymbol{r},\omega) \right],$$

which can be solved by setting to zero the kernel in curly brackets. This yields the desired relation between the potentials:

$$v_{\mathrm{SF}}(\boldsymbol{r},\omega) = v^h_{\mathrm{SF}}\big(\omega - c(\boldsymbol{r},\omega)\big) + c(\boldsymbol{r},\omega) - v_{\mathrm{e}}(\boldsymbol{r}) - v_{\mathrm{H}}(\boldsymbol{r}).$$

## III. ALUMINUM

Aluminum shows a similar performance of our connector approach with respect to a standard SE calculation as sodium. The results are presented in Fig. 3: as for Na, both the SF and the BS are very well reproduced, and just the bandwidth is slightly underestimated: while the expected SE result is 12.65 eV and a DFT approach with the PBE GGA[3] results in a bandwidth of 11.09 eV (12.3% off the SE result), the value obtained with our theory is 12.43 eV (1.7% off): as for Na, our approach leads to a huge improvement over KS.

## IV. PLAIN LDA CONNECTOR

In this section we will give a quick overview of the performance of three connectors that are simpler than the one considered in the main article.

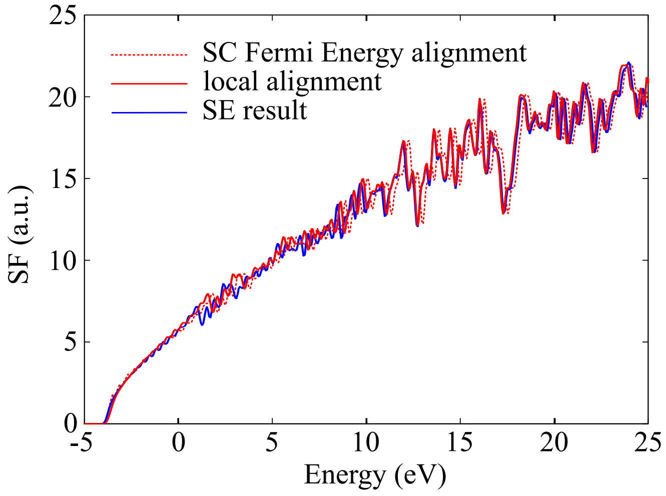


FIG. 4: Sodium SF, in atomic units, as a function of frequency, with $\mu$ set to zero. The blue curve is the SE, the dotted red one for eq. (6) with a self-consistent Fermi energy, and the continuous red line for the local alignment of eq. (7).

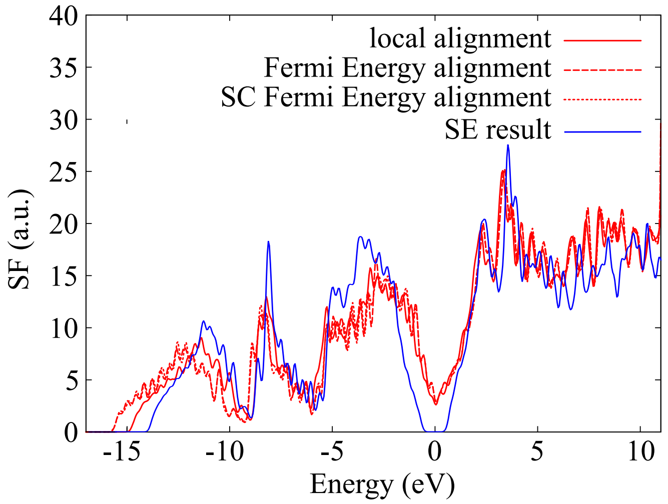


FIG. 5: Silicon SF, in atomic units, as a function of frequency. The blue curve is the SE, while the red ones are the three simpler connector approaches: the dashed one for eq. (6) with the Fermi energy taken from the reference calculation; the dotted one with a self consistent procedure, and the continuous line for the local alignment of eq. (7). While the reference SE curve is plotted with its midgap aligned to the zero of the frequency axis, the red curves have no gap, and the comparison is just qualitative.

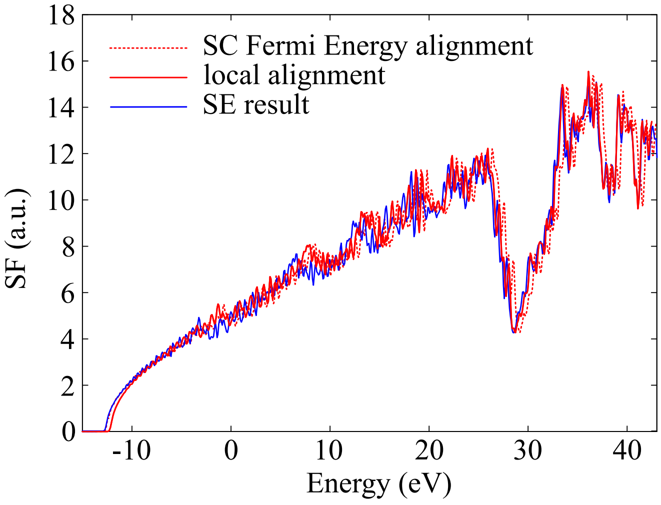


FIG. 6: Aluminum SF, in atomic units, as a function of frequency, with $\mu$ aligned with the zero. The blue curve is the SE, the dotted red one for eq. (6) with a self-consistent Fermi energy, and the continuous red line for the local alignment of eq. (7).

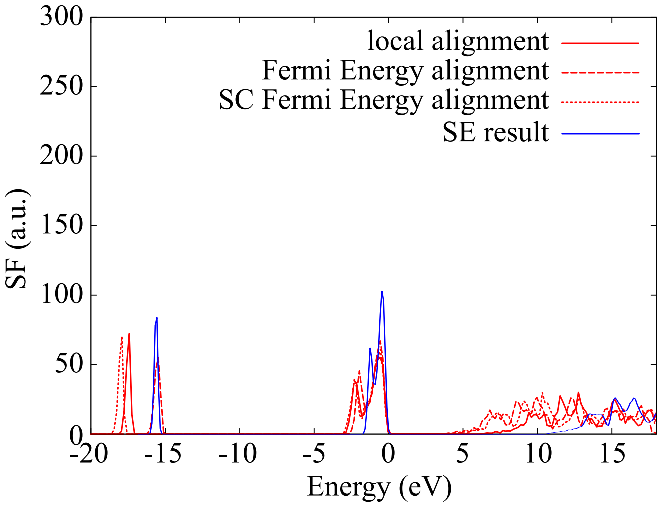


FIG. 7: Argon SF, in atomic units, as a function of frequency, with $\mu$ aligned with the zero. The blue curve is the SE, while the red ones stand for the three simple connector approaches: the dashed one for eq. (6) with the Fermi energy taken from the reference calculation; the dotted one with a self consistent procedure, and the continuous line for the local alignment of eq. (7).

The first one is a plain LDA-type connector, where for each point in space $\boldsymbol{r}$ a HEG with the local density $n(\boldsymbol{r})$ is built, and the zero of frequency is set by aligning the Fermi energies of the real system $\mu$ and the local-HEG $\mu^h = \mu^h[n(\boldsymbol{r})]$:

$$v_{\rm SF}(\boldsymbol{r},\omega) = v^h_{{\rm SF}|n^h=n(\boldsymbol{r})}\left(\omega - \mu + \mu^h(\boldsymbol{r})\right). \qquad (6)$$

The Fermi energy of the real material $\mu$ can be set in various ways. Here we consider two possibilities: first, using the one of the reference calculation, or second, by an iteration cycle: one first guesses a value $\mu^{(\rm in)}$, plugs it into Eq. (6), performs the calculation and evaluates the resulting Fermi energy $\mu^{(\rm out)}$, which becomes the new input parameter for the second cycle, until convergence is reached. For the materials we considered this procedure is converging after a few steps.

To avoid passing through the Fermi energy, we also replaced the difference $\mu - \mu^h(\boldsymbol{r})$ with the sum of the exter-

nal and the Hartree potential; this trade is in principle justified for slowly varying density[4]; the corresponding potential of this third simple connector is:

$$v_{\rm SF}(\boldsymbol{r},\omega) = v^{h}_{{\rm SF}|n^h=n(\boldsymbol{r})}\left(\omega - v_{\rm e}(\boldsymbol{r}) - v_{\rm H}(\boldsymbol{r})\right). \quad (7)$$

The results of these simpler connectors for the four prototypical materials we have considered are presented in Figs. 4, 5, 6, and 7. For the metals Na and Al, although the overall agreement is good, the position of the peaks at low energy (in particular the ones at 0.85 eV and 2.60 eV for Na and the ones at 6.28 eV and 13 eV for Al) is overestimated. Concerning Si, none of the three simple connectors is able to open a gap, and the width of the last four occupied bands is too large. The same behavior shows up in Ar, where the gap is strongly underestimated while the bandwidth is overestimated.

These examples show the necessity of going beyond the simpler connectors of Eq. (6) or Eq. (7) towards, for instance, the dynLCA considered in the main article.

## V. TECHNICAL DETAILS

For studying real materials, we have employed the open source package `abinit`[5], version 7.10.5. There, an HSE06 hybrid[6] calculation is already implemented, with a screening length of 9.090909 $a_0$. For testing our approach, we have replaced the usual SE construction with the reading of our external HEG database; we have then perturbatively performed a QP calculation using the SP instead of the SE.

To obtain the SF by integrating the BS, each QP delta peak has been replaced by a gaussian function, with a broadening of 0.1 eV.

In the following we give the parameters we used for producing the results presented in the paper.

**Sodium** BCC lattice, with experimental[7] lattice constant $a$ =4.225Å. We employed a Trouiller-Martins (TM) pseudopotential[8]. For the three calculations, LDA, SE and dynLCA, we used a Γ-centered grid of $30 \times 30 \times 30$ $k$-points, making 752 $k$-points in the irreducible Brillouin zone, and 20 bands. Common cut-off energy of 20.0 Hartree (Ha), and a gaussian smearing of 0.01 Ha. For the SE calculation, a cutoff of 4.0 Ha in the exchange part of it, and 6.0 Ha for the wavefunctions.

**Aluminium** FCC lattice, lattice constant $a$ =4.049Å. Optimized norm-conserving Vanderbilt (ONCV) pseudopotential[9]. Γ-centered grid of $38 \times 38 \times 38$ $k$-points, making 1440 $k$-points in the irreducible Brillouin zone, and 20 bands. Cutoff energy of 20.0 Ha, and a temperature smearing of 0.005 Ha. For the SE calculation, a cutoff of 4.0 Ha in the exchange part of it, and 6.0 Ha for the wavefunctions.

**Silicon** FCC lattice, experimental[7] lattice constant $a$ =5.429Å. TM pseudopotential[8]. Monkhorst-Pack[10] of $14 \times 14 \times 14$ $k$-points with 4 shifts, making 344 $k$-points in the irreducible Brillouin zone, and 12 bands. Cutoff energy of 20.0 Ha. For the SE calculation, a cutoff of 4.0 Ha in the exchange part of it, and 10.0 Ha for the wavefunctions.

**Argon** FCC lattice, experimental[7] lattice constant $a$ =5.256Å. TM pseudopotential[8]. Monkhorst-Pack[10] grid of $12 \times 12 \times 12$ $k$-points with 4 shifts, making 231 $k$-points in the irreducible Brillouin zone, and 12 bands. Cutoff energy of 20.0 Ha. For the SE calculation, a cutoff of 12.0 Ha in the exchange part of it, and 16.0 Ha for the wavefunctions.

* marco.vanzini@polytechnique.edu


1 L. J. Sham and M. Schlüter, Phys. Rev. Lett. **51**, 1888 (1983).
2 M. Gatti, V. Olevano, L. Reining, and I. V. Tokatly, Phys. Rev. Lett. **99**, 057401 (2007).
3 J. P. Perdew, K. Burke, and M. Ernzerhof, Phys. Rev. Lett. **77**, 3865 (1996).
4 L. J. Sham and W. Kohn, Phys. Rev. **145**, 561 (1966).
5 X. Gonze, G.-M. Rignanese, M. Verstraete, J.-M. Beuken, Y. Pouillon, R. Caracas, F. Jollet, M. Torrent, G. Zerah, M. Mikami, *et al.*, Z. Kristallogr **220**, 558 (2005).
6 J. Heyd, G. E. Scuseria, and M. Ernzerhof, The Journal of Chemical Physics **124**, 219906 (2006).
7 R. Wyckoff, *Crystal structures*, 2nd ed., Vol. 1 (Interscience Publishers, New York, 1963).
8 N. Troullier and J. L. Martins, Phys. Rev. B **43**, 1993 (1991).
9 D. R. Hamann, Phys. Rev. B **88**, 085117 (2013).
10 H. J. Monkhorst and J. D. Pack, Phys. Rev. B **13**, 5188 (1976).
